# Supplementary material for: Real-world K-Anonymity Applications: the \textsc{KGen} approach and its evaluation in Fraudulent Transactions
Source: arXiv:2204.01533 source file (2026-07-21)
Supplement: Supplementary file 1 [file APPENDIX_A.tex]

\clearpage
\appendix
\section{APPENDIX A: \textsc{KGen} User manual}

The \textsc{KGen} approach provides a command user interface that allows to execute basic functions. From the github repository (https://github.com/danieldp92/\textsc{KGen}), it is possible to download the jar file (or the source file and build the relative jar file) and execute the program. Being written in Java, it must be run using the following command:

\begin{lstlisting}
  java -jar \textsc{KGen}.jar <option>
\end{lstlisting}

\vspace{0.6cm}

The options available can be checked with the option -h (or --help). There are four different options:

\begin{itemize}
    \item \texttt{-a --algorithm}: Choose an algorithm for the anonymization of a dataset. It's possible to choose 4 algorithms: EXHAUSTIVE, OLA, \textsc{KGen}, RANDOM. 
    
    \textbf{Command line format:} \texttt{-a <algorithmName> <threshold> <datasetPath> <configPath>}
    
    \textbf{Output:} the dataset anonymized
    
    \item \texttt{-e --experimentation}: Run the entire experimentation, comparing all the algorithms available in the tool. You can set the number of runs, in order to run multiple times all meta-heuristic approaches. 
    
    \textbf{Command line format:} \texttt{-e <numberOfRuns> <threshold> <datasetPath> <configPath>} 
    
    \textbf{Output:} Results and statistics in CVS format, in order to extract all information for the evaluation study.
    
    \item \texttt{-s --stat}: Run the stat generator. From results generated by an experimentation, this option allows you to compute relevant statistical information.
    
    \textbf{Command line format:} \texttt{-s <resultPath>} 
    
    \textbf{Output:} Statistics from input results in csv.
    
    \item \texttt{-c --config}:  Generate a config file, that it's necessary to start the algorithm.
    
    \textbf{Command line format:} \texttt{-c <datasetPath>}
    
    \textbf{Output:} the config file needed for the anonymization
    
    \item \texttt{-o --output}:  This is optional. If you add this option at the end of the command line, you can change the output file.
    
    \textbf{Command line format:} \texttt{-o <outputPath>}
\end{itemize}

The tool realized supports four different techniques, already discussed in the evaluation chapter \ref{sec:evaluation}, viz.: EXHAUSTIVE, OLA, \textsc{KGen} and RANDOM approaches. With this tool it is possible to select the technique of choice to be executed.

For the anonymization process, you obviously need to have the dataset to anonymize, the configuration file, and, the threshold of the maximum erasable rows allowed, in floating point (for example a threshold of 0.5 is equals to 50\%).

\subsection{Configuration file}

The configuration file specifies the attributes.

Basically, we can define two categories of meta-data associated to the attributes: 
\begin{itemize}
    \item \textbf{Identifiers / Quasi-Identifiers:} we need to know if an attribute is an identifiers or a quasi identifiers. The difference is that an identifiers will be completely anonymized in the process. Instead a quasi-identifiers will be partially anonymized. So, if the data related to this attribute is not absolutely unique and you want to preserve as much as possible the utility, just set it as quasi-identifiers;
    \item \textbf{Data type:} another important information about the attribute is the type. There are five different types: Data, Integer, String, Place, Double. Each of these types has a different generalization strategy. So, the choice of the type influences the anonymization strategy on that type.
\end{itemize}

\subsection{Tool examples}
In this section we provide some screen example of our tool. If you don't know how to execute a command, you can use the help option, as shown in the Fig. \ref{fig:demo_help}.

The main usage of the tool revolves around the algorithm option. Its usage is shown in Fig. \ref{fig:demo_algorithm}. The Fig. \ref{fig:demo_execution_cl} shows how to write the command:

\vspace{-0.6cm}

\begin{lstlisting}
  java -jar \textsc{KGen}.jar -a \textsc{KGen} 0.005 
        <datasetPath> <configPath>
\end{lstlisting}

Using this command line will be executed the \textsc{KGen} algorithm with a maximum suppression level of 0.5\%. The running example is whown in Fig. \ref{fig:demo_execution_pb}. If you don't have the configuration file, you can create it with this command:

\vspace{-0.6cm}

\begin{lstlisting}
  java -jar \textsc{KGen}.jar -c <datasetPath>
\end{lstlisting}

The default output path is the same path of the jar file. However, if you want to change it, you can put the output option at the end of the command. For example, this command:

\vspace{-0.6cm}

\begin{lstlisting}
  java -jar \textsc{KGen}.jar -c <datasetPath>
        -o outputPath<>
\end{lstlisting}

generate a configFile and save it in the output path indicated.

\begin{figure*}[h]
    \centering
    \includegraphics[width = .8\linewidth]{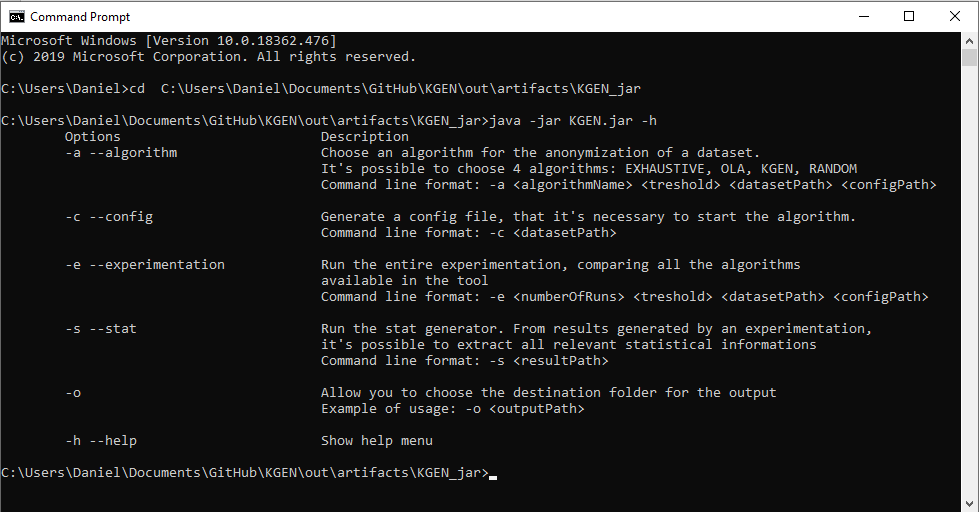}
    \vspace{0.5cm}
    \caption{Help screen}
    \label{fig:demo_help}
\end{figure*}
\begin{figure*}[h]
    \centering
    \begin{subfigure}{\linewidth}
        \centering
        \includegraphics[width = .8\linewidth]{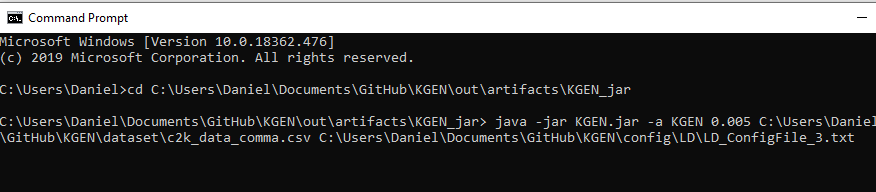}
        \caption{Command line example for the anonymization of a dataset.}
        \label{fig:demo_execution_cl}        
    \end{subfigure}
    
    \vspace{0.5cm}
    
    \begin{subfigure}{\linewidth}
        \centering
        \includegraphics[width = .8\linewidth]{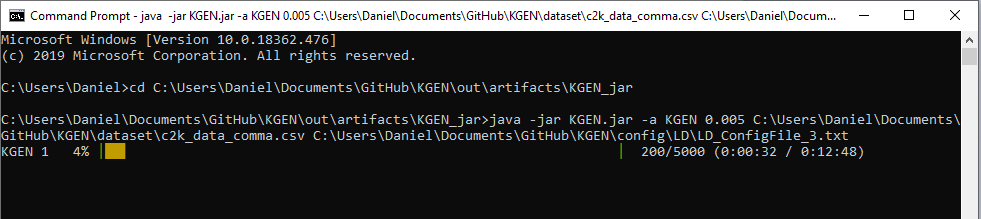}
        \caption{Execution of the tool.}
        \label{fig:demo_execution_pb}        
    \end{subfigure}

    \vspace{0.5cm}
    
    \caption{Anonymization command example}
    \label{fig:demo_algorithm}
\end{figure*}
