# Supplementary material for: Real-world K-Anonymity Applications: the \textsc{KGen} approach and its evaluation in Fraudulent Transactions
Source: arXiv:2204.01533 source file (2026-07-21)
Supplement: Supplementary file 2 [file demo_execution.tex]

\begin{figure*}[h]
    \centering
    \begin{subfigure}{\linewidth}
        \centering
        \includegraphics[width = .8\linewidth]{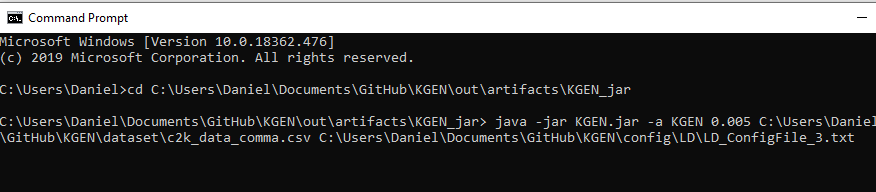}
        \caption{Command line example for the anonymization of a dataset.}
        \label{fig:demo_execution_cl}        
    \end{subfigure}
    
    \vspace{0.5cm}
    
    \begin{subfigure}{\linewidth}
        \centering
        \includegraphics[width = .8\linewidth]{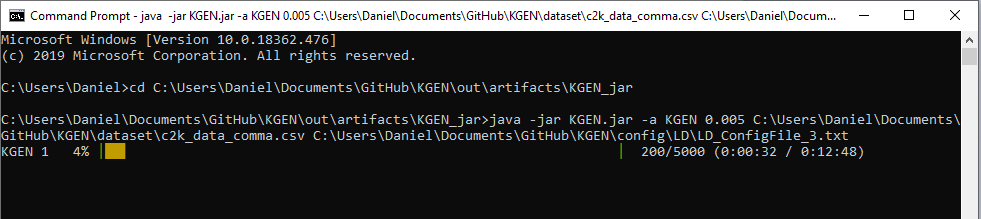}
        \caption{Execution of the tool.}
        \label{fig:demo_execution_pb}        
    \end{subfigure}

    \vspace{0.5cm}
    
    \caption{Anonymization command example}
    \label{fig:demo_algorithm}
\end{figure*}
