# Supplementary material for: Real-world K-Anonymity Applications: the \textsc{KGen} approach and its evaluation in Fraudulent Transactions
Source: arXiv:2204.01533 source file (2026-07-21)
Supplement: Supplementary file 3 [file demo_help.tex]

\begin{figure*}[h]
    \centering
    \includegraphics[width = .8\linewidth]{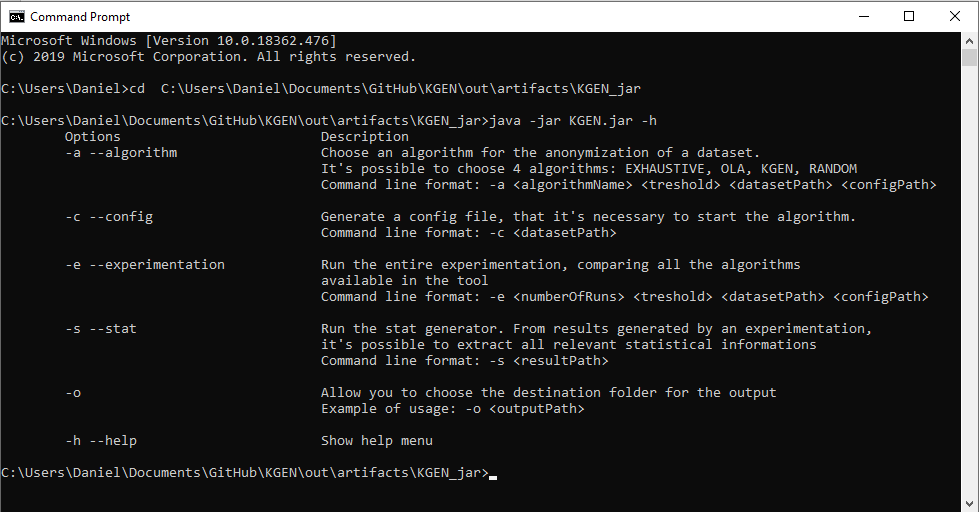}
    \vspace{0.5cm}
    \caption{Help screen}
    \label{fig:demo_help}
\end{figure*}
